# Supplementary material for: Dynamic Multi-Behavior Sequence Modeling for Next Item Recommendation
Source: arXiv:2301.12105 source file (2023-01-28)
Supplement: Supplementary file 1 [file 999appendix.tex]

\section{Experiments}
\subsection{Experimental Settings}
\subsubsection{Datasets}
\begin{table}[h]
\centering
\fontsize{9}{10.8}\selectfont
\begin{tabular}{l|ccc}
% \hline
%                   & Taobao                 & Tmall                      & E-commerce               \\ \hline
% \#Users            & 987,994 (99,793)       & 424,170 (200,531)          & 13,334,687 (251,331)     \\
% \#Items            & 4,162,024 (596,382)    & 1,090,390 (89,008)         & 3,477,502 (79,235)       \\
% \#Purchases        & 2,015,839 (726,627)    & 3,292,144 (1,960,910)      & 6,510,474 (2,752,725)    \\
% \#Favorites        & 2,888,258 (319,134)    & 3,005,723 (1,254,927)      & -                        \\
% \#Add-to-carts     & 5,530,446 (730,094)    & 76,750 (20,882)            & 15,283,350 (4,343,451)   \\
% \#Clicks           & {\fontsize{6.4}{9}\selectfont  89,716,264 (9,879,402)} & {\fontsize{6.4}{9}\selectfont 48,550,713 (12,197,927)}    & {\fontsize{6.4}{9}\selectfont 158,567,115 (26,879,537)} \\
% Time period        & 9 days                 & 186 days                   & 32 days                  \\
% Year               & 2017                   & $\le$2014                  & 2021                     \\ \hline
\hline
                  & Taobao                 & Tmall                      & GS Retail              \\ \hline
\#Users            & 987,994                & 424,170                   & 13,334,687 \\
\#Items            & 4,162,024              & 1,090,390                 & 3,477,502 \\
\#Purchases        & 2,015,839              & 3,292,144                 & 6,510,474 \\
\#Favorites        & 2,888,258              & 3,005,723                 & -         \\
\#Add-to-carts     & 5,530,446              & 76,750                    & 15,283,350 \\
\#Clicks           & 89,716,264             & 48,550,713                & 158,567,115 \\
Time period        & 9 days                 & 186 days                   & 32 days                  \\
Year               & 2017                   & $\le$2014                  & 2021                     \\ \hline
\end{tabular}
\caption{Statistics of datasets.} %The numbers in parenthesis indicate the remaining ones after filtering out the users/items with few interactions.}
\label{table:statistics}
\end{table}

Table \ref{table:statistics} provides the detailed statistics of the datasets. 
In our experiments, for all datasets, we filtered out users and items that have less than five interactions on the target behavior (i.e., Purchase) as done in previous works \cite{hmgcr,ehcf}, and used recent 500 interactions of each user. 
\begin{itemize}
    \item \textbf{Taobao}\footnote{https://tianchi.aliyun.com/dataset/dataDetail?dataId=649} is a dataset offered by Alibaba, and contains user behaviors in four types: Purchase, Add-to-cart, Favorite, and Click. The dataset was collected for 9 days in 2017, and also provides the item category information. 
    \item \textbf{Tmall}\footnote{https://tianchi.aliyun.com/dataset/dataDetail?dataId=47} is a dataset accumulated by Tmall.com, about the users' multi-behaviors for six months: Purchase, Add-to-cart, Favorite, and Click. The description of this dataset does not provide the year information of data, but it was collected before 2015, because this dataset was released in 2015. 
    \item \textbf{GS Retail} is a new, large and up-to-date dataset we release in this paper. The user behavior data of GS shop, which is an e-commerce and home shopping brand of GS Retail, was collected for a month in 2021. 
    This dataset contains three types of user behaviors: Purchase, Add-to-cart, and Click. Compared with the other datasets, this dataset has the largest and the most up-to-date data about the user behaviors. 
\end{itemize}

\subsubsection{Evaluation}
To evaluate the recommendation performance of each model, we used the most recent interacted item on the target behavior of each user as the test item, and the second most recent one as the validation item, and trained the model with the rest of the data. 
The test performance was reported with the best model when the validation performance was the best, that is, when the validation performance did not improved for 10 consecutive epochs. 

\subsubsection{Baselines}
\begin{itemize}
    \item \textbf{Single-behavior-based methods}
    \begin{itemize}
        \item \textbf{BPR-MF} \cite{bpr} is a matrix factorization method, with a pair-wise loss for personalized ranking. 
        \item \textbf{GRU4Rec} \cite{gru4rec} uses GRU to encode a sequence of item embedding into the final representation.
        \item \textbf{SASRec} \cite{sasrec} captures the user interests in a item sequence using a self-attentive network. 
        \item \textbf{FMLP-Rec} \cite{fmlp}, which is one of the state-of-the-art SRSs, utilizes an all-MLP structure and filtering algorithms to denoise the item sequence data. 
    \end{itemize}
    \item \textbf{Multi-behavior-based methods}
    \begin{itemize}
        \item \textbf{METAS} \cite{metas} designs the relationships between users and items in an action space and an entity space, and learns them with multi-task metric learning. 
        \item \textbf{EHCF} \cite{ehcf} learns user-item relationships with transfer learning between the behaviors, a non-sampling optimization method and multi-task learning. 
        \item \textbf{HMG-CR} \cite{hmgcr} adopts graph neural networks based on hyper meta-paths between a user's behaviors, and a graph contrastive learning between them.
        \item \textbf{CML} \cite{cml} uses contrastive meta network to model the cross-type behavior dependencies. 
        \item \textbf{MBN} \cite{mbn} is a multi-behavior SRS that uses a RNN-based meta multi-behavior sequence encoder to capture meta-knowledge between multi-behavior sequences and a recurring-item-aware predictor.
        \item \textbf{TGT} \cite{tgt} is a multi-behavior SRS that captures short-term user interests with a behavior-aware transformer network and long-term user interests via a temporal graph neural network. 
        \item \textbf{\proposedA} is a light version of the proposed method which dynamically integrates the capsules encoding each behavior sequence with dynamic routing, considering the characteristics of multi-behavior sequences. 
        \item \textbf{\proposedB} is an improved version of the proposed method, which applies the dynamic routing even to encoding each behavior sequence using dynamic GRU to capture the dynamic correlation between the multi-behavior sequences. 
    \end{itemize}
\end{itemize}

\subsubsection{Implementation Details}
We implemented the methods with PyTorch 1.11 on Ubuntu 20.04. 
We conducted all experiments on a machine with a 16-core Intel Xeon Gold 6226R 2.9GHz CPU, an NVIDIA RTX A5000 24GB GPU and a 384GB RAM. 
We used Adam optimizer \cite{adam} to optimize all models, and tuned the hyperparameters based on the validation N@10 performance: learning rate $\eta \in \{0.01, 0.003, 0.001, 0.0003, 0.0001\}$, dropout rate $p \in \{0.0, 0.1, 0.2, 0.3, 0.4, 0.5\}$, coefficient for L2 regularization $\lambda \in \{0.0, 0.001, 0.01, 0.1\}$, embedding dimension $D \in \{16, 32, 64, 128\}$, batch size $\mathcal{B} \in \{64, 128, 256, 512\}$, and the number of negative samples $\in \{1, 2, 4, 8\}$ for the methods that require negative sampling. 
For SRSs, we tuned the length of sequence  $\mathcal{L} \in \{10, 20, 50, 100\}$. 
Other hyperparameters for the baselines were tuned in the ranges provided in their papers. 

\subsection{Performance Comparison}
Table 4 provides the performance of the single-behavior-based methods.
\begin{table}[h]
\centering
\fontsize{9}{10.8}\selectfont
\setlength{\tabcolsep}{1.3pt}
\begin{tabular}{c|c|cccc}
\hline
Dataset                     & Metric & BPR-MF & GRU4Rec & SASRec & FMLP-Rec \\ \hline
\multirow{6}{*}{\rotatebox[origin=c]{90}{Taobao}}     & H@10   & 0.0414 & 0.0190  & 0.0409 & 0.0464   \\
                            & H@20   & 0.0487 & 0.0225  & 0.0431 & 0.0489   \\
                            & N@10   & 0.0264 & 0.0136  & 0.0347 & 0.0412   \\
                            & N@20   & 0.0282 & 0.0144  & 0.0352 & 0.0418   \\ \cline{2-6} 
                            & \#Prm  & 89.1M  & 153.4M  & 19.1M  & 38.2M    \\
                            & Inf.t  & 17.4   & 15.8    & 14.1   & 15.6     \\ \hline
\multirow{6}{*}{\rotatebox[origin=c]{90}{Tmall}}      & H@10   & 0.0101 & 0.0067  & 0.0093 & 0.0092   \\
                            & H@20   & 0.0170 & 0.0104  & 0.0130 & 0.0131   \\
                            & N@10   & 0.0050 & 0.0039  & 0.0064 & 0.0062   \\
                            & N@20   & 0.0068 & 0.0048  & 0.0073 & 0.0072   \\ \cline{2-6} 
                            & \#Prm  & 37.1M  & 23.0M   & 5.7M   & 5.8M     \\
                            & Inf.t  & 4.3    & 5.6     & 5.1    & 6.0      \\ \hline
\multirow{6}{*}{\rotatebox[origin=c]{90}{GS Retail}} & H@10   & 0.0329 & 0.1028  & 0.1225 & 0.1081   \\
                            & H@20   & 0.0485 & 0.1247  & 0.1399 & 0.1322   \\
                            & N@10   & 0.0174 & 0.0741  & 0.0992 & 0.0766   \\
                            & N@20   & 0.0214 & 0.0796  & 0.1036 & 0.0827   \\ \cline{2-6} 
                            & \#Prm  & 42.3M  & 20.4M   & 2.5M   & 5.1M     \\
                            & Inf.t  & 7.0    & 5.2     & 5.5    & 6.9      \\ \hline
\end{tabular}
\caption{Overall performance of single-behavior-based methods on the next item prediction.}
\label{table:single}
\end{table}

\subsection{Analyses on \proposedA and \proposedB}
\subsubsection{Hyperparameter Study}
Fig. 5 and 6 shows the N@10 performance of \proposedA and \proposedB with various combinations of $r$ and $l$ on Tmall, GS Retail, relatively. 

\begin{figure}[h]
    \centering
    % \fbox{\includegraphics[width=0.5\columnwidth, trim={2.0cm 2.2cm 2.0cm 3.0cm}, clip] {figures/hyperparameter_example.pdf}}
    \begin{subfigure}[b]{0.38\columnwidth}
        \centering
        \includegraphics[width=\textwidth] {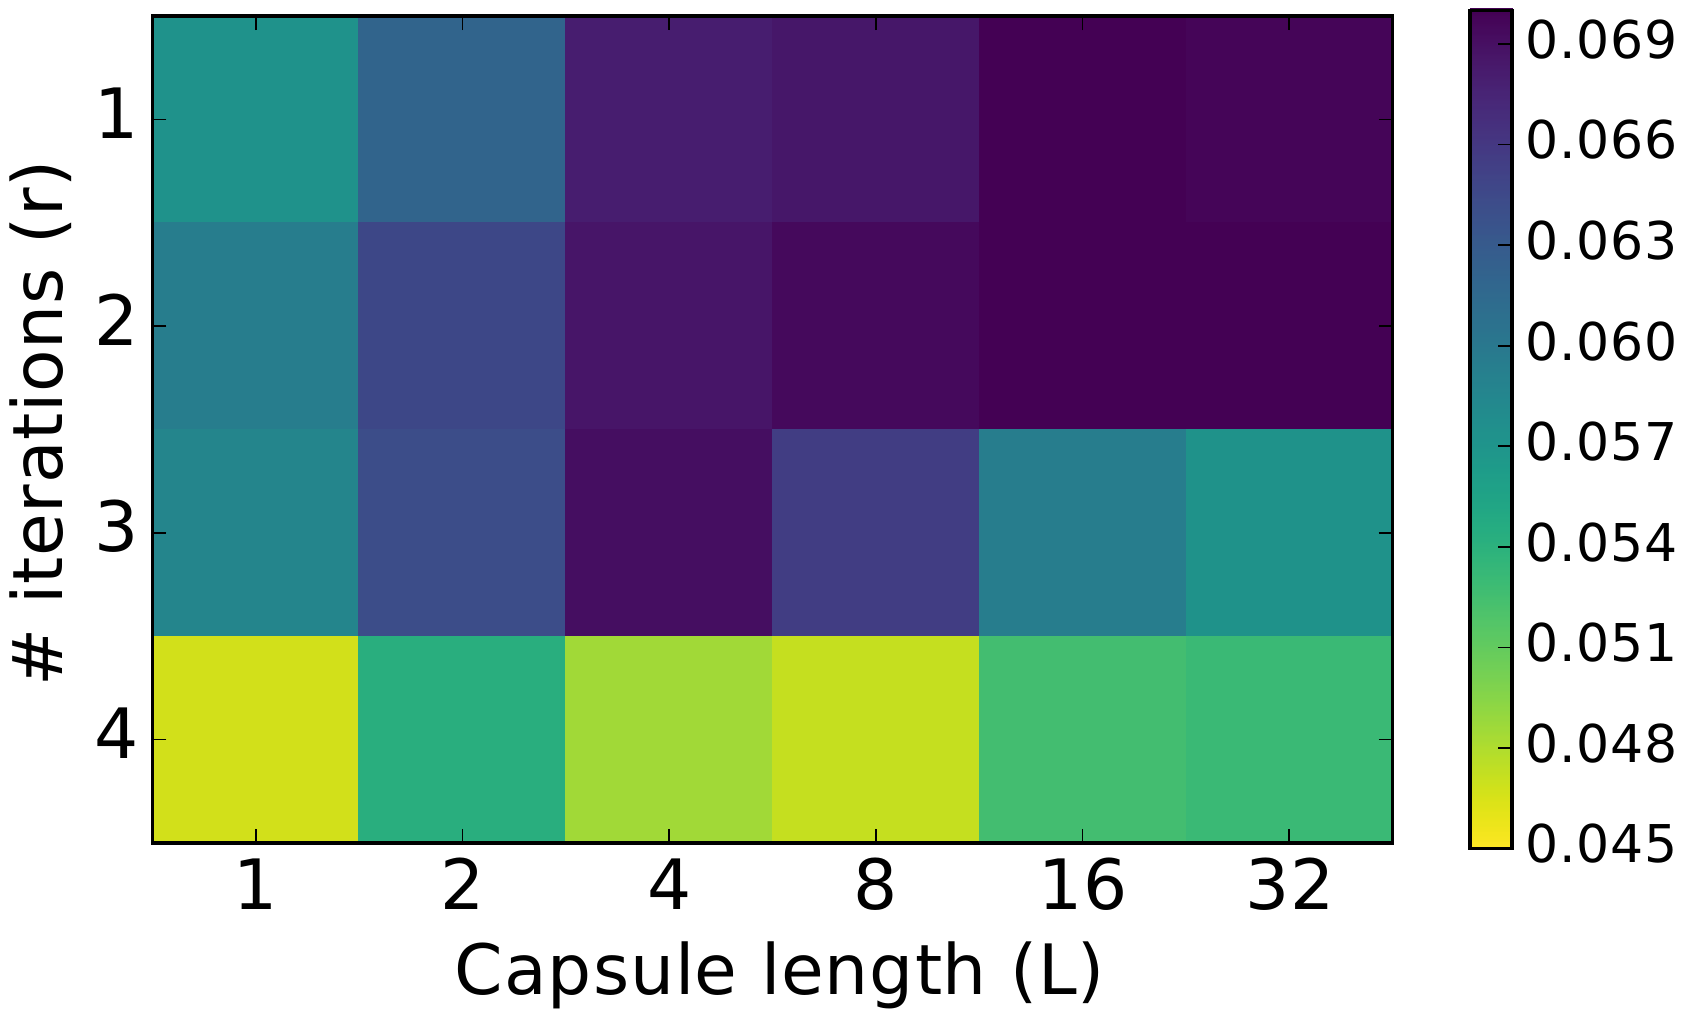}
        \caption{\proposedA}
    \end{subfigure}
    \begin{subfigure}[b]{0.38\columnwidth}
        \centering
        \includegraphics[width=\textwidth] {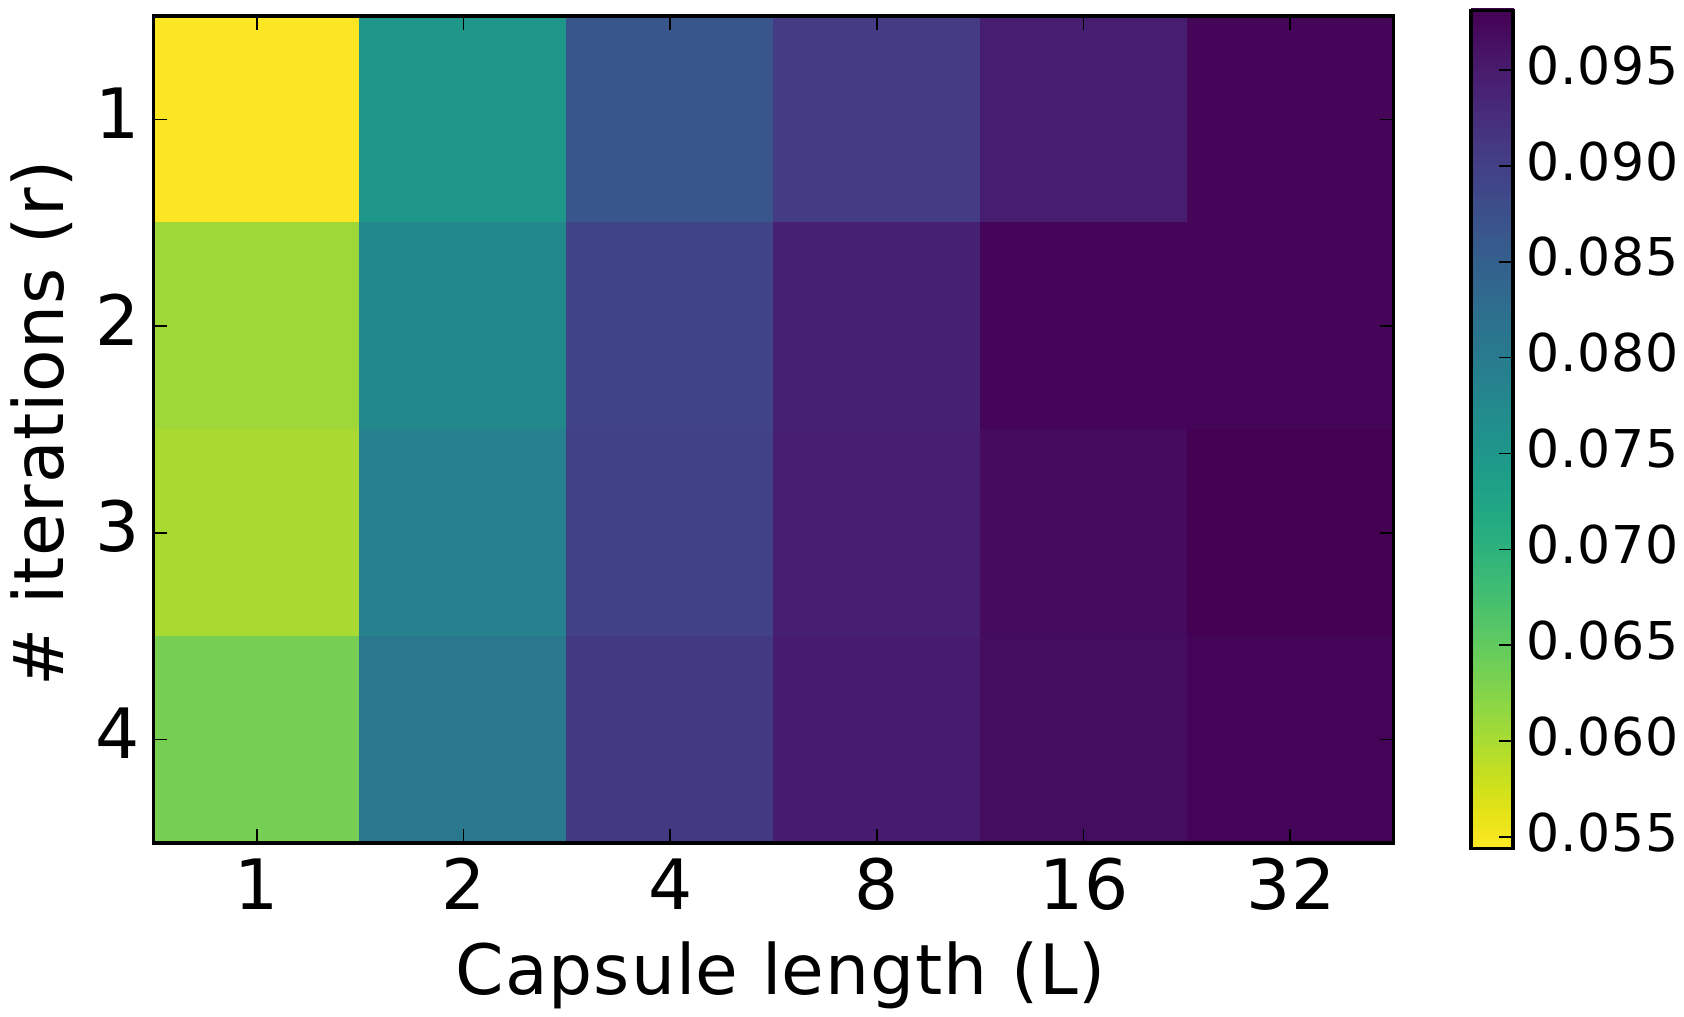}
        \caption{\proposedB}
    \end{subfigure}
    \caption{N@10 performance on Tmall with various combinations of the capsule length and the number of iterations.}
    \label{fig:hyperparameter_tmall}
\end{figure}

\begin{figure}[h]
    \centering
    % \fbox{\includegraphics[width=0.5\columnwidth, trim={2.0cm 2.2cm 2.0cm 3.0cm}, clip] {figures/hyperparameter_example.pdf}}
    \begin{subfigure}[b]{0.38\columnwidth}
        \centering
        \includegraphics[width=\textwidth] {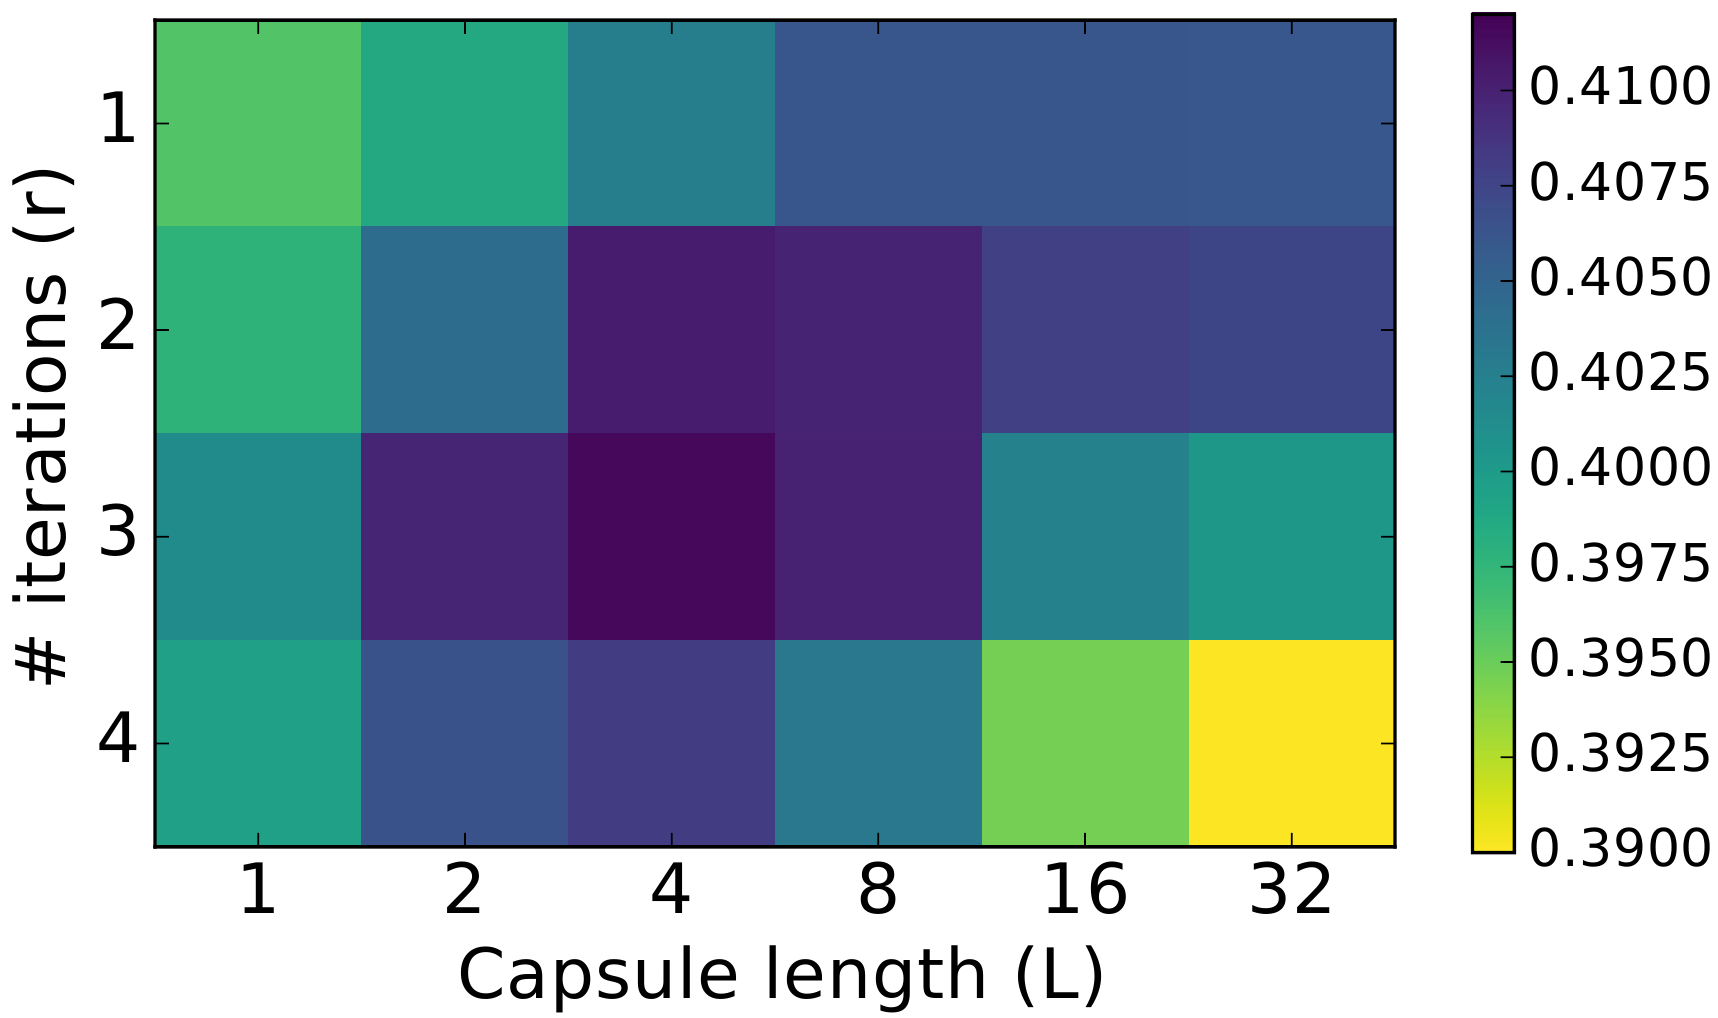}
        \caption{\proposedA}
    \end{subfigure}
    \begin{subfigure}[b]{0.38\columnwidth}
        \centering
        \includegraphics[width=\textwidth] {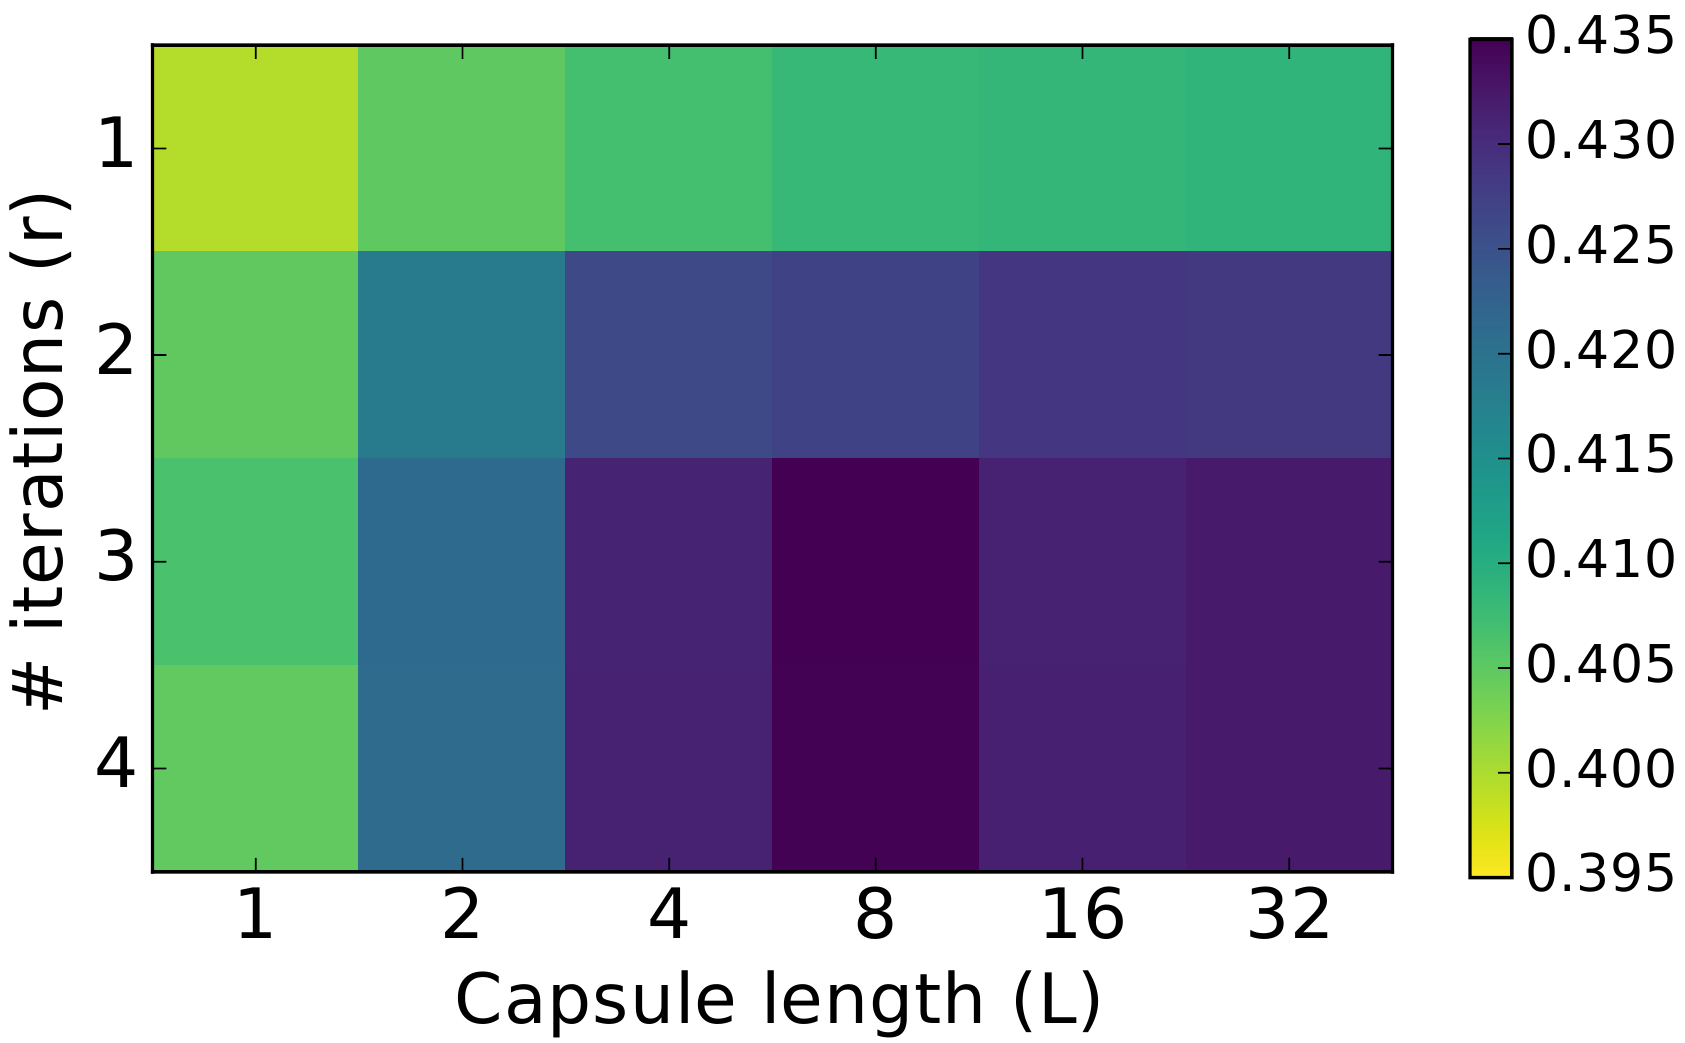}
        \caption{\proposedB}
    \end{subfigure}
    \caption{N@10 performance on GS Retail with various combinations of the capsule length and the number of iterations.}
    \label{fig:hyperparameter_ecommerce}
\end{figure}

\subsubsection{Analysis on Dynamic Routing}
We analyse the effectiveness of the dynamic routing in \proposedB, which is applied to the dynamic GRU. % for each behavior sequence. 
% to change the state of each input item based on the correlations between sequences.
%% dynamic GRU의 목적은 현재 sequence의 item들의 state가 다른 sequence들의 내용에 따라 바뀌고, correlation에 따라 중요한 item을 더 중요하게 인코딩하는 것이다. 
In other words, this analysis aims to show that the state of items in a behavior sequence changes based on the contents of other sequences via the dynamic routing, so that important items are encoded with more attention according to the correlations between the sequences. 
Fig. \ref{fig:dymus_plus} shows the result of a case study with a trained \proposedB with $r=4$, when we replace the last item in a random user's Click sequence in Taobao with a random item in the same category as a specific item in the user's Purchase sequence. 
Each value represents the change of the importance of each input item within the user's Purchase sequence compared to before the replacement. % when encoding it with the dynamic GRU.
We represent the importance change as the change rate of cosine similarity between the new gate (i.e., $\mathbf{N}^{(l)}_k$) for each input item in the Purchase sequence and the final hidden state (i.e., $\mathbf{H}^{(l)}_{t^b}$) of the dynamic GRU for Purchase. 
If \proposedB determines that a purchased item is important considering the correlations between the sequences, it will encode the item with more attention, and the cosine similarity will increase.
As a result, the dynamic routing in \proposedB reflects the importance of the recently \textit{clicked} item to the Purchase sequence and encodes the related item with high importance, which shows the superiority of \proposedB in modeling the correlations at item-level. 
\begin{figure}[h]
    \centering
    \includegraphics[width=0.69\columnwidth]{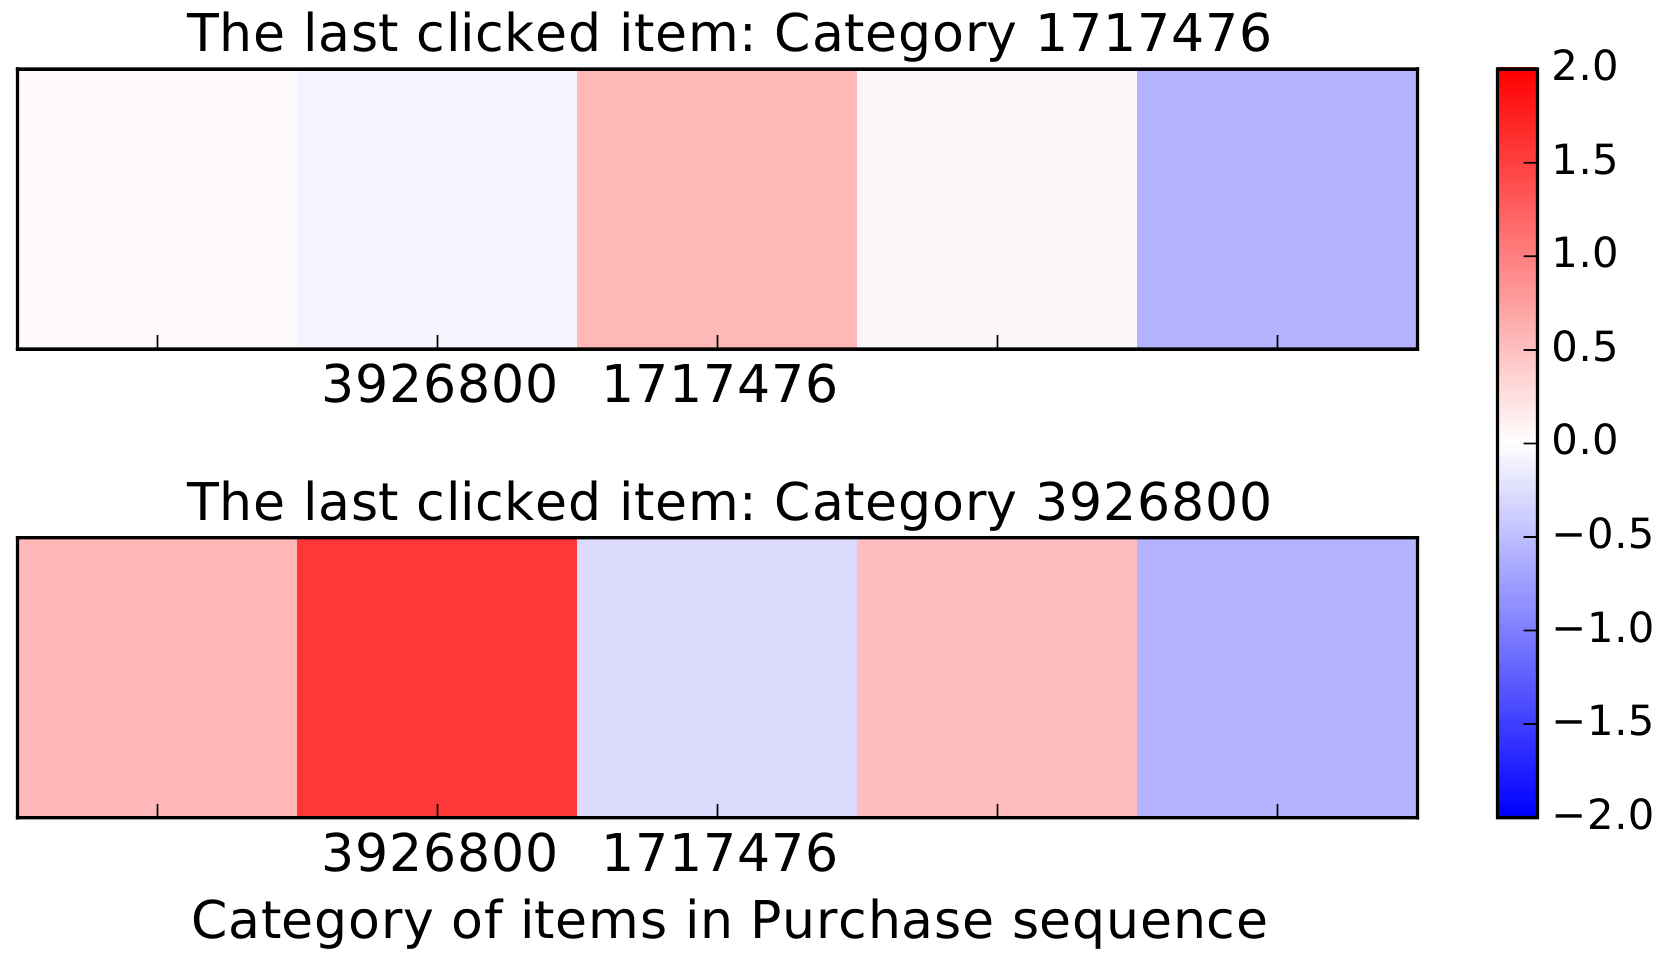}
    % \caption{The change rate in cosine similarity between each new gate and the final hidden state of the dynamic GRU of a user's Purchase sequence on Taobao after replacing the last clicked item (for the last five items).}
    \caption{The importance change of each of the last five items in the user's Purchase sequence, when replacing the last clicked item.}
    \label{fig:dymus_plus}
\end{figure}

\subsubsection{Ablation Study}
The results of ablation studies on Tmall and GS Retail are reported in Table 5 and 6, respectively.

\begin{table}[h]
\centering
\fontsize{9}{10.8}\selectfont
\setlength{\tabcolsep}{1.3pt}
\begin{tabular}{c|c|cc|cccc}
\hline
            & Original & Sum    & Self-att & -P     & -A     & -F     & -C     \\ \hline
\proposedA  & 0.0694   & 0.0635 & 0.0639   & 0.0663 & 0.0562 & 0.0686 & 0.0369 \\
\proposedB  & 0.0941   & 0.0692 & 0.0786   & 0.0725 & 0.0817 & 0.0926 & 0.0488 \\
MBN         & 0.0630   & -      & -        & 0.0617 & 0.0623 & 0.0635 & 0.0041 \\ \hline

\end{tabular}
\caption{Ablation study on Tmall (N@10).}
\label{table:ablation_tmall}
\end{table}

\begin{table}[h]
\centering
\fontsize{9}{10.8}\selectfont
\setlength{\tabcolsep}{1.3pt}
\begin{tabular}{c|c|cc|cccc}
\hline
            & Original & Sum    & Self-att & -P     & -A     & -F     & -C     \\ \hline
\proposedA  & 0.4103   & 0.3651 & 0.3741   & 0.3172 & 0.3397 & \ \quad-\ \quad\quad & 0.2381 \\
\proposedB  & 0.4270   & 0.3986 & 0.4030   & 0.3219 & 0.3406 & - & 0.2607 \\
MBN         & 0.3443   & -      & -        & 0.3365 & 0.2915 & - & 0.2184 \\ \hline

\end{tabular}
\caption{Ablation study on GS Retail (N@10).}
\label{table:ablation_ecommerce}
\end{table}
